# Supplementary material for: Parallel and Asynchronous Smart Contract Execution
Source: arXiv:2306.05007 source file (2023-06-08)
Supplement: Supplementary file 1 [file appendix.tex]

\atc{
\section{Communication Pattern in BFT Protocols}

\begin{figure}[htbp]
\centering
\begin{tikzpicture}
  [scale=.6,auto=center]
   \node at (1.1, 5.5) {\scriptsize \sf request};
   \node at (3, 5.5) {\scriptsize \sf pre-prepare};
   \node at (5, 5.5) {\scriptsize \sf prepare};
    \node at (7, 5.54) {\scriptsize \sf commit};
     \node at (9, 5.5) {\scriptsize \sf reply};

   \draw [thick, dotted] (1.9, 0.5) -- (1.9, 6);
    \draw [thick, dotted] (4.1, 0.5) -- (4.1, 6);
     \draw [thick, dotted] (6, 0.5) -- (6, 6);
      \draw [thick, dotted] (8, 0.5) -- (8, 6);

   \node at (0,5) {$\Cli$};
   \draw [thick] (0.5,5) -- (10,5);
   \draw [->,shorten >=2pt,>=stealth] (0.6, 5) -- (1.9, 4);

    \node at (0,4) {$\Ser_1$};
     \draw [thick] (0.5,4) -- (10,4);
     \draw [->,shorten >=2pt,>=stealth] (2.1, 4) -- (3.9, 3);
     \draw [->,shorten >=2pt,>=stealth] (2.1, 4) -- (3.8, 2);
     \draw [->,shorten >=2pt,>=stealth] (2.1, 4) -- (3.85, 1);

     \draw [->,shorten >=2pt,>=stealth] (6.1, 4) -- (7.9, 3);
     \draw [->,shorten >=2pt,>=stealth] (6.1, 4) -- (7.6, 2);
     \draw [->,shorten >=2pt,>=stealth] (6.1, 4) -- (7.4, 1);

     \draw [->,shorten >=2pt,>=stealth] (8.1, 4) -- (9.5, 5);

   \node at (0,3) {$\Ser_2$};
   \draw [thick] (0.5,3) -- (10,3);
     \draw [->,shorten >=2pt,>=stealth] (4.1, 3) -- (5.3, 4);
     \draw [->,shorten >=2pt,>=stealth] (4.1, 3) -- (5.8, 2);
     \draw [->,shorten >=2pt,>=stealth] (4.1, 3) -- (5.5, 1);

     \draw [->,shorten >=2pt,>=stealth] (6.3, 3) -- (7.5, 4);
     \draw [->,shorten >=2pt,>=stealth] (6.3, 3) -- (7.8, 2);
     \draw [->,shorten >=2pt,>=stealth] (6.3, 3) -- (7.7, 1);

      \draw [->,shorten >=2pt,>=stealth] (8.4, 3) -- (9.6, 5);

    \node at (0,2) {$\Ser_3$};
  \draw [thick] (0.5,2) -- (10,2);
     \draw [->,shorten >=2pt,>=stealth] (4.1, 2) -- (5.5, 4);
     \draw [->,shorten >=2pt,>=stealth] (4.1, 2) -- (5.6, 3);
     \draw [->,shorten >=2pt,>=stealth] (4.1, 2) -- (5.9, 1);

     \draw [->,shorten >=2pt,>=stealth] (6.2, 2) -- (7.7, 4);
     \draw [->,shorten >=2pt,>=stealth] (6.2, 2) -- (7.6, 3);
     \draw [->,shorten >=2pt,>=stealth] (6.2, 2) -- (7.99, 1);

     \draw [->,shorten >=2pt,>=stealth] (8.2, 2) -- (9.8, 5);

    \node at (0,1) {$\Ser_4$};
    \draw [thick] (0.5,1) -- (10,1);
    \node at (1.5, 1) {$\xmark$};

%\draw [decorate,decoration={brace,amplitude=5pt}]
(2,6) -- (8,6) node %[black,midway,yshift=8]
%{\scriptsize {\bf Agreement}};

\end{tikzpicture}
        \caption{Communication pattern in PBFT~\cite{PBFT}.}
        \label{fig:PBFT}
\end{figure}

\remove{
\begin{figure}[htbp]
    \label{fig:Zyzzyva}
    \centering
    \begin{subfigure}[Fast track.]
    {
\begin{tikzpicture}[scale=0.6]
    \node at (0.9, 5.5) {\scriptsize \sf request};
    \node at (3, 5.5) {\scriptsize \sf preprepare};
    \node at (5.1, 5.5) {\scriptsize \sf reply};

    \draw [thick, dotted] (1.85, 0.5) -- (1.85, 6);
    \draw [thick, dotted] (4.15, 0.5) -- (4.15, 6);

   \node at (-0.5,5) {$\Cli$};
   \draw [thick] (0,5) -- (6.5,5);
   \draw [->,shorten >=2pt,>=stealth] (0.1, 5) -- (1.9, 4);

    \node at (-0.5,4) {$\Ser_1$};
    \draw [thick] (0,4) -- (6.5,4);
    \draw [->,shorten >=2pt,>=stealth] (2.1, 4) -- (3.9, 3);
    \draw [->,shorten >=2pt,>=stealth] (2.1, 4) -- (3.8, 2);
    \draw [->,shorten >=2pt,>=stealth] (2.1, 4) -- (3.9, 1);

   \node at (-0.5,3) {$\Ser_2$};
   \draw [thick] (0,3) -- (6.5,3);

   \draw [->,shorten >=2pt,>=stealth] (4.2, 3) -- (5.5, 5);

    \node at (-0.5,2) {$\Ser_3$};
    \draw [thick] (0,2) -- (6.5,2);

    \draw [->,shorten >=2pt,>=stealth] (4.3, 2) -- (5.7, 5);

    \node at (-0.5,1) {$\Ser_4$};
    \draw [thick] (0,1) -- (6.5,1);
    \draw [->,shorten >=2pt,>=stealth] (4.4, 1) -- (5.9, 5);
    
\end{tikzpicture}
        \label{fig:fast_zyzzyva}
    %    \vspace{-0.8 em}
    }\end{subfigure}
    \hfill
    \begin{subfigure}[Two-phase track.]
    {
\begin{tikzpicture}[scale=.6]
    \node at (0.9, 5.5) {\scriptsize \sf request};
    \node at (3, 5.5) {\scriptsize \sf preprepare};
    \node at (5.1, 5.5) {\scriptsize \sf reply};
    \node at (8, 5.55) {\scriptsize \sf commit};

    \draw [thick, dotted] (1.85, 0.5) -- (1.85, 6);
    \draw [thick, dotted] (4.15, 0.5) -- (4.15, 6);
    \draw [thick, dotted] (6, 0.5) -- (6, 6);
  %  \draw [thick, dotted] (8, -2.5) -- (8, 6);

   \node at (-0.5,5) {$\Cli$};
   \draw [thick] (0,5) -- (10,5);
   \draw [->,shorten >=2pt,>=stealth] (0.1, 5) -- (1.9, 4);

    \node at (-0.5,4) {$\Ser_1$};
    \draw [thick] (0,4) -- (10,4);
    \draw [->,shorten >=2pt,>=stealth] (2.1, 4) -- (3.9, 3);
    \draw [->,shorten >=2pt,>=stealth] (2.1, 4) -- (3.8, 2);
    \draw [->,shorten >=2pt,>=stealth] (2.1, 4) -- (3.9, 1);

    \draw [->,shorten >=2pt,>=stealth] (6, 5) -- (7.9, 3);
    \draw [->,shorten >=2pt,>=stealth] (6, 5) -- (7.8, 2);
    \draw [->,shorten >=2pt,>=stealth] (6, 5) -- (7.7, 1);

   \node at (-0.5,3) {$\Ser_2$};
   \draw [thick] (0,3) -- (10,3);

    \draw [->,shorten >=2pt,>=stealth] (4.2, 3) -- (5.7, 5);
    \draw [->,shorten >=2pt,>=stealth] (8.1, 3) -- (9.7, 5);

    \node at (-0.5,2) {$\Ser_3$};
    \draw [thick] (0,2) -- (10,2);

    \draw [->,shorten >=2pt,>=stealth] (4.3, 2) -- (5.9, 5);
    \draw [->,shorten >=2pt,>=stealth] (8.2, 2) -- (9.9, 5);

    \node at (-0.5,1) {$\Ser_4$};
    \draw [thick] (0,1) -- (10,1);
    \node at (1.5, 1) {$\xmark$};
    
\end{tikzpicture}
        \label{fig:twophase_zyzzyva}
    %    \vspace{-0.8 em}
    }\end{subfigure}
    \caption{Communication pattern in Zyzzyva~\cite{Zyzzyva}.}
\end{figure}
}

\begin{figure}[htbp]
\centering
\begin{tikzpicture}
  [scale=.6,auto=center]
   \node at (1.1, 5.5) {\scriptsize \sf request};
   \node at (3, 5.5) {\scriptsize \sf pre-prepare};
   \node at (5.5, 5.5) {\scriptsize \sf prepare};
    \node at (8.5, 5.54) {\scriptsize \sf commit};
     \node at (10.7, 5.5) {\scriptsize \sf reply};

   \draw [thick, dotted] (1.9, 0.5) -- (1.9, 6);
    \draw [thick, dotted] (4.1, 0.5) -- (4.1, 6);
     \draw [thick, dotted] (7, 0.5) -- (7, 6);
      \draw [thick, dotted] (10, 0.5) -- (10, 6);

   \node at (0,5) {$\Cli$};
   \draw [thick] (0.5,5) -- (11.5,5);
   \draw [->,shorten >=2pt,>=stealth] (0.6, 5) -- (1.9, 4);

    \node at (0,4) {$\Ser_1$};
     \draw [thick] (0.5,4) -- (11.5,4);
     \draw [->,shorten >=2pt,>=stealth] (2.1, 4) -- (3.9, 3);
     \draw [->,shorten >=2pt,>=stealth] (2.1, 4) -- (3.8, 2);
     \draw [->,shorten >=2pt,>=stealth] (2.1, 4) -- (3.85, 1);
     
    \draw [->,shorten >=2pt,>=stealth] (5.6, 4) -- (6.9, 3);
    \draw [->,shorten >=2pt,>=stealth] (5.6, 4) -- (6.8, 2);
    \draw [->,shorten >=2pt,>=stealth] (5.6, 4) -- (6.85, 1);

     \draw [->,shorten >=2pt,>=stealth] (8.6, 4) -- (9.9, 3);
     \draw [->,shorten >=2pt,>=stealth] (8.6, 4) -- (9.6, 2);
     \draw [->,shorten >=2pt,>=stealth] (8.6, 4) -- (9.4, 1);

     \draw [->,shorten >=2pt,>=stealth] (10.1, 4) -- (11.2, 5);

   \node at (0,3) {$\Ser_2$};
   \draw [thick] (0.5,3) -- (11.5,3);
     \draw [->,shorten >=2pt,>=stealth] (4.1, 3) -- (5.3, 4);

     \draw [->,shorten >=2pt,>=stealth] (7.3, 3) -- (8.5, 4);

      \draw [->,shorten >=2pt,>=stealth] (10.4, 3) -- (11.3, 5);

    \node at (0,2) {$\Ser_3$};
  \draw [thick] (0.5,2) -- (11.5,2);
     \draw [->,shorten >=2pt,>=stealth] (4.1, 2) -- (5.5, 4);

     \draw [->,shorten >=2pt,>=stealth] (7.2, 2) -- (8.6, 4);

     \draw [->,shorten >=2pt,>=stealth] (10.5, 2) -- (11.45, 5);

    \node at (0,1) {$\Ser_4$};
    \draw [thick] (0.5,1) -- (11.5,1);
    \node at (1.5, 1) {$\xmark$};

%\draw [decorate,decoration={brace,amplitude=5pt}]
(2,6) -- (8,6) node %[black,midway,yshift=8]
%{\scriptsize {\bf Agreement}};

\end{tikzpicture}
        \caption{Communication pattern in ByzCoin (ByzCoinX)~\cite{Byzcoin,Omniledger}.}
        \label{fig:ByzCoin}
\end{figure}

\remove{
\subsection{Correctness argument for \BFT} %\dawn{should we use some better term than "argument"?}}
\label{sec:argument}

\subsubsection{Safety argument}
We informally argue that if a correct server $\Ser_i$ executes a transaction $\trans$ with a sequence number $sn$ in view $v$, then no correct server executes a different transaction with the same sequence number in view $v' \geq v$.

The intuition behind this arguement is that if $\Ser_i$ executes $\trans$ with $sn$ in view $v$, it must have seen either of the follows:
\begin{enumerate}
\item $\langle \prepared, H(M), sn, v, \widetilde{\sigma}_1 \rangle$ (line~\ref{13} in Figure~\ref{fig:saberBFT_normal_case}). 
In this case, all $3f+1$ servers must have received the corresponding $\preprepareM$ message. 
\begin{enumerate}
    \item Before switching to the next view, no correct server will execute a different transaction with the same $sn$, since they will not accept a different $\preprepareM$ with $sn$ from the current primary.
    \item Recall that they are required to receive at least $2f+1$ $\viewchangeM$ messages to switch to the next view, then there will be at least $f+1$ correct servers include that $\preprepareM$ in their message logs. That means if they switch to the next view, either line~\ref{2.9}, line~\ref{2.11} or line~\ref{2.13} in \fig~\ref{fig:SaberBFT_view_change} will happen. If line~\ref{2.9} happens, correct servers will execute $\trans$ before switching to the next view. If line~\ref{2.11} happens, given that there will not be a $\commitrequestM$ message for a different transaction with a view number higher than or equal to $v$, correct servers will commit and execute $\trans$ in the next view. Same for line~\ref{2.13}. %It is possible that there are at most $f$ correct servers are isolated so that they cannot switch to the next view. However, they will not switch to different views and execute different transactions either, because they are less than $2f+1$ even adding the $f$ faulty servers. 
\end{enumerate}

\item $\langle \committed, M, sn, v, \widetilde{\sigma}_2, \widetilde{\sigma}'_2 \rangle$ (line~\ref{26} in \fig~\ref{fig:saberBFT_normal_case}). In this case, at least $2f+1$ servers must have received the corresponding $\preprepareM$ and $\commitrequestM$ messages. 
\begin{enumerate}
    \item Before switching to the next view, no correct server will execute a different transaction with the same  $sn$, since only at most $f$ servers will accept a different $\preprepareM$ message with $sn$.
    \item There will be at least one correct server including that $\commitrequestM$ message in its message log. That means if they switch to the next view, either line~\ref{2.9}, line~\ref{2.11} or line~\ref{2.15} in \fig~\ref{fig:SaberBFT_view_change} will happen. Due to the same reason as case 1.b), all correct servers will execute $\trans$ with $sn$ before or after switching to the next view.
\end{enumerate}
%\item both.
\end{enumerate}

\subsubsection{Liveness argument}
We say that $\Cli$'s request {\em completes} once $\Cli$ accepts the reply.
We say a view is {\em stable} if the primary is correct and no asynchrony. 
We informally argue that a transaction requested by a correct client eventually completes.
The intuition behind this argument is as follows:
\begin{enumerate}
    \item In a stable view, %where the primary $\Ser_p$ is correct,
    a valid $\preprepareM$ message will be sent, a valid $\committedM$ message will be formed, and all correct servers will reply \mbox{to $\Cli$.}
    %Unless asynchrony occurs among correct correct servers (e.g., cannot build a $\commited$ message because at least one correct server is isolated), $\Cli$'s request will be completed within this view.
    \item If the view is unstable and view-change happens. Suppose a quorum $Q$ of $2f+1$ correct replicas requests a view-change. We distinguish between three cases:
    \begin{enumerate}
        \item The new primary $\Ser_{p'}$ is correct and all replicas in $Q$ received a valid $\newviewM$ message. They will change to a stable view successfully %(\fig{}, line~\ref{}).

        \item None of the correct replicas received a valid $\newviewM$ message. In this case, another view-change will start.

        \item Only a quorum $Q'$ of less than $2f + 1$ correct replicas received a valid $\newviewM$ message. In this case, faulty replicas can follow the protocol to make the correct replicas in $Q'$ change to a non-stable view. %Other correct replicas will send new $\reqviewchange$ messages due to timeout, but a view-change will not start since they are less than $f+1$. 
        When faulty replicas deviate from the protocol, the correct replicas in $Q'$ will \mbox{trigger a new view-change.}
    \end{enumerate}
    In cases b) and c), a new view-change triggers the system to one of the above three cases again. Under a weak synchrony assumption, messages are guaranteed to be delivered in polynomial time. Therefore, the system will eventually reach case a), i.e., a stable view will be reached.
\end{enumerate}
}
}

\section{Correctness arguments for SaberCryptoKitties}
\label{sec:security_ethereum}

%\ray{Do we have anything more formal? If so, we can point to it. If not, we shouldn't use the phrase "informally argue".}
%\dawn{should we move this to the appendix?}
We informally show that the transaction $\trans$ invoking {\em giveBirth\_lock} will lead to the same state transition as invoking {\em giveBirth}, 
on condition that there are (more than) $f'+1$ $\exec$s in each execution committee, which is enforced by the {\em Shuffle} function. 
The {\em giveBirth\_lock} function checks the validity of $\trans$ (same as {\em giveBirth}), 
lock the required states and designate only one committee for the execution of $\trans$. 
The required states will keep being locked until the {\em giveBirth\_unlock} function being invoked, 
which requires a multisignature from the designated committee.
Note that the multisignature $\widetilde{\sigma}$ is associated with $\trans$, 
so signatures for other transactions cannot be used for $\trans$.
Furthermore, there will {\em not} be two (or more) multisignatures with different {\em childGenes} from that group, 
because there is at least one correct $\exec$ that will not sign twice.
Therefore, the {\em giveBirth\_unlock} function for $\trans$ can only be invoked with one possible {\em childGenes}, 
which leads to the same state as {\em giveBirth} achieves. 
A subtle difference is the order of the {\em kitties}, because there may be other kitties generated between {\em giveBirth\_lock} and {\em giveBirth\_unlock}. 
However, this will not affect the safety.
%is the same as {\em giveBirth}.
%Once {\em giveBirth\_unlock} completes, the state is the same as {\em giveBirth} completes.

\section{Correctness arguments for $\name$}
\label{sec:correctness_saberledger}

%\dawn{should we move this to appendix?}
\Paragraph{Safety.} We informally show that the global state of the blockchain will not diverge after one round (thus it will never diverge), 
on condition that %there are (more than) $3f+1$ $\order$s 
the consensus layer is secure
and $f'+1$ $\exec$s in each group, 
which is enforced by the randomness beacon and epoch transitions. 
If a state $\st$ diverges into two different states $\st'$ and $\st''$, then either (or both) of the following cases happens: 
\begin{enumerate}
    \item $\st'$ and $\st''$ are returned by the same group;
    \item $\st'$ and $\st''$ are returned by two different groups;
\end{enumerate}

In case 1), that group must have returned two valid multisignatures $\widetilde{\sigma}'$ and $\widetilde{\sigma}''$, each of which are aggregated from ($f'+1$) $\exec$s' outputs. 
Then, there are must be at least one correct $\exec$ in that group outputs both $\st'$ and $\st''$, which will never happen.

In case 2), both groups must have received $\st$, 
which means the consensus layer has put $\st$ into two different transactions blocks, which will never happen 
%An honest $\order_p$ will never do this.
%If $\order_p$ is faulty, this behavior will be detected by other $\order$s and view-change will happen (cf. Section~\ref{sec:view-change}). 

%An honest $\order_{p}$ will eventually be chosen. 

\Paragraph{Liveness.} 
Since the consensus layer is live and there are $f'+1$ replicas in each execution group, the protocol will keep running. 
%as long as $\order_p$ and all committee leaders are correct. 
%The liveness property of the underlying BFT protocol ensures that a faulty $\order_p$ will be replaced. 
%A faulty committee leader will be replaced by its successors.
